# Supplementary material for: Discriminative Semantic Transitive Consistency for Cross-Modal Learning
Source: arXiv:2103.14103 source file (2022-03-20)
Supplement: Supplementary file 1 [file ablation_hyper_supple.tex]

\section{Ablation of Hyperparameters}
\label{sec:ablation_hyperparameter}
We experimented with wide range of hyperparameters and picked the one that performs best in the val set. We also observe that the performance remains similar for most of the hyperparameters values. We give the results for \texttt{Sentence Pascal} dataset in Tab.~\ref{tab:hyperparameter} below. We observe from the results that the performance is quite stable for different values of the hyperparameters and the results doesn't change significantly. From this observation, we conclude that the approach is not much sensitive to the value of hyperparameters.
\begin{table}[!htbp]
    \centering
    % \resizebox{.9\columnwidth}{!}{
    % \renewcommand{\arraystretch}{0.4}
    \scalebox{1.0}{
    \begin{tabular}{cccc|ccc}
    \hline
    $\alpha$&$\beta$&$\gamma$&$\delta$ & I2T & T2I & Both\\
    \hline \hline
    10.0 & 1.0 & 0.01 &   0.1 & 0.6923 & 0.7092 & 0.7007\\
    10.0 & 1.0 & 0.01 &   0.0 & 0.6959 & 0.7095 & 0.7027\\
    10.0 & 1.0 & 0.01 &   1.0 & 0.6985 & 0.7104 & 0.7044\\
    10.0 & 1.0 & 0.01 &  10.0 & 0.6897 & 0.7028 & 0.6963\\
    \hline
    10.0 & 1.0 & 0.1 &  0.1 & 0.6944 & 0.7087 & 0.7016\\
    10.0 & 1.0 & 0.1 &  0.0 & 0.6954 & 0.7044 & 0.6999\\
    10.0 & 1.0 & 0.1 &  1.0 & 0.6974 & 0.7017 & 0.6996\\
    10.0 & 1.0 & 0.1 & 10.0 & 0.6882 & 0.7045 & 0.6963\\ 
    \hline
    10.0 & 1.0 & 1.0 &  0.1 & 0.6959 & 0.7059 & 0.7009\\
    10.0 & 1.0 & 1.0 &  0.0 & 0.6963 & 0.7021 & 0.6992\\
    10.0 & 1.0 & 1.0 &  1.0 & 0.6989 & 0.7063 & 0.7026\\
    10.0 & 1.0 & 1.0 & 10.0 & 0.6888 & 0.7031 & 0.6959\\
    \hline
    10.0 & 1.0 & 10.0 &  0.1 & 0.6918 & 0.7020 & 0.6969\\
    10.0 & 1.0 & 10.0 &  0.0 & 0.6914 & 0.7065 & 0.6989\\
    10.0 & 1.0 & 10.0 &  1.0 & 0.6938 & 0.7023 & 0.6981\\
    10.0 & 1.0 & 10.0 & 10.0 & 0.6915 & 0.6994 & 0.6954\\
    \hline
    1.0 & 1.0 & 0.01 &   0.1 & 0.6827 & 0.6954 & 0.6890\\
    1.0 & 1.0 & 0.01 &   0.0 & 0.6763 & 0.7082 & 0.6922\\
    1.0 & 1.0 & 0.01 &   1.0 & 0.6856 & 0.6968 & 0.6912\\
    1.0 & 1.0 & 0.01 &  10.0 & 0.6843 & 0.6998 & 0.6920\\
    \hline
    1.0 & 10.0 & 0.01 &   0.1 & 0.6924 & 0.6820 & 0.6872\\
    1.0 & 10.0 & 0.01 &   0.0 & 0.6761 & 0.6812 & 0.6786\\
    1.0 & 10.0 & 0.01 &   1.0 & 0.6640 & 0.6996 & 0.6818\\
    1.0 & 10.0 & 0.01 &  10.0 & 0.6630 & 0.6876 & 0.6753\\
    \hline \hline
    \end{tabular}
    }
    % \vspace{-1 em}
    \caption{Ablation Study: Contribution of different hyperparameter for retrieval in \texttt{Sentence Pascal} dataset}
    \label{tab:hyperparameter}
    % \vspace{-1 em}
\end{table}
